# Supplementary material for: An Interpretable and Sparse Neural Network Model for Nonlinear Granger Causality Discovery
Source: arXiv:1711.08160 source file (2018-06-25)
Supplement: Supplementary file 1 [file appendix_ts.tex]

\section{Appendix}
To optimize Problems (\ref{gp_mlp}) and (\ref{hg}) we utilize proximal gradient ascent. Specifically, if we let $\Omega({\bf W})$ denote the sparsity enducing penalty, then the proximal algorithm starts at $k = 1$ and iterates
\begin{align}
{\bf W}^{k + 1} =  P_{\lambda \Omega} ({\bf W}^k + \gamma \nabla L(x_{1:T},{\bf W} ) ) \nonumber
\end{align}
where $L(x_{1:T},{\bf W} ) = \sum_{t = 1}^T \left(x_{ti} - g_i(x_{(t-1):(t-K)}, { \bf W}) \right)^2$ is the MLP loss function , $\gamma \in (0, 1)$ is a step size, and $P_{\lambda \Omega}$ is the proximal function for $\Omega$. Since both group and heirarchical penalties only effect the input layer weights, the weights for other layers are not affected by the proximal step. 

For ease of notation, let the matrix $\tilde{W}^{1j} = (W^{11}_{:j}, \ldots, W^{1K}_{:j})$.  For the group lasso penalty the proximal function decomposes across encoding weights for each series $j$ and is given by
\begin{align}
P_{\lambda \Omega}(\tilde{W}^j) = \begin{cases} 
0 \,\,\,\,\, &\text{if } || \tilde{W}^j||_F < \lambda \\
\left(1 - \frac{\lambda}{||\tilde{W}^j||_F} \right) \tilde{W}^j & \text{otherwise.} \nonumber
\end{cases} 
\end{align}
For the heirarchical penalty the proximal operation is given by recursively applying group lasso proximal operators across the nested groups \cite{}:
For more details on proximal methods see \cite{}.
